# Supplementary material for: Laparoscopic Scene Analysis for Intraoperative Visualisation of Gamma Probe Signals in Minimally Invasive Cancer Surgery
Source: arXiv:2501.01752 source file (2025-01-03)
Supplement: Supplementary file 1 [file code_listing.tex]

\clearpage
