# Supplementary material for: Laparoscopic Scene Analysis for Intraoperative Visualisation of Gamma Probe Signals in Minimally Invasive Cancer Surgery
Source: arXiv:2501.01752 source file (2025-01-03)
Supplement: Supplementary file 2 [file appendix.tex]

\chapter*{Appendices}
\chaptermark{Appendices}
\addcontentsline{toc}{chapter}{Appendices}

\begin{cabstract}
The GitHub repository at \url{https://github.com/mlnotebook} contains the code used in this work as well as those snippets shown here.
\end{cabstract}

\begin{enumerate}[wide, labelindent=1cm, label=\textbf{Listing \arabic*:}]
\itemsep0.4cm 
\item Add two Integers in Python.
\end{enumerate}

\vspace*{\fill}
\clearpage
\clearpage
